# Supplementary material for: Indian Political Twitter and Caste Discrimination -- How Representation Does Not Equal Inclusion in Lok Sabha Networks
Source: arXiv:2007.15863 source file (2020-07-31)
Supplement: Supplementary file 1 [file appendix.tex]

\newpage

\appendix

\section{Pairwise odds ratios}
\label{appendix}

Table \ref{table:uppervslower} shows the odds of getting retweeted by the \upperc MPs for each pair of castes, the odds ratio and the statistical significance of the difference in ratio using Fisher's exact test. For brevity, we show the results of only those pairs that have significant differences. 

\begin{table}[ht]
\centering
\resizebox{\textwidth}{!}{
\begin{tabular}{l|llllll}
\toprule
\textbf{Party} & \textbf{caste1} & \textbf{odds of caste1} & \textbf{caste2} &  \textbf{Odds of caste2} &  \textbf{Odds Ratio} & \textbf{p-value} \\
\midrule
BJP & \ucb & 1.667 & \ic & 1.080 & 1.543 & 0.001 \\
 & \ucb & 1.667 & \obc & 0.991 & 1.682 & 0.000 \\
 & \ucb & 1.667 &  \scs & 0.682 & 2.444 & 0.000 \\
 & \ucb & 1.667 &  \st  & 0.476 & 3.502 & 0.000 \\
 & \ucb & 1.667 & \ucnb & 1.283 & 1.299 & 0.007 \\
 & \ucnb & 1.283 & \obc  & 0.991 & 1.295 & 0.049\\
 & \ucnb & 1.283 &  \scs & 0.682 & 1.882 & 0.006 \\
 & \ucnb & 1.283 & \st & 0.476 & 2.695 & 0.007 \\ 
 & \ic & 1.080 & \st & 0.476 & 2.268 & 0.028 \\
 \bottomrule
Non-BJP & \ucb & 2.625 & \scs & 0.214 & 12.250 & 0.000 \\
 & \ucnb & 1.636 & \scs & 0.214 & 7.636 & 0.004\\
 & \ic & 2.286 & \scs & 0.214 & 10.667 & 0.000 \\
 & \obc & 1.383 & \scs & 0.214 & 6.454 & 0.002 \\ \bottomrule
\end{tabular}
}
\caption{\textbf{The second column, caste1, denotes the caste with higher odds of getting retweeted by \upperc than caste2 in fourth column. Odds ratio in the penultimate column is the proportion of odds of caste1 to that of caste2, and the last column denotes the p-value of the Fisher's exact test. The significance level is kept at 0.05 and all numbers are rounded to 3 decimal places.}}
\label{table:uppervslower}
\end{table}

Table \ref{table:samevsdiff} compares for each pair of castes the odds of getting retweeted by their own caste. Similar to Table \ref{table:uppervslower}, we show the results of only those pairs that have significant differences. 

\begin{table}[ht]
\centering
\resizebox{\textwidth}{!}{
\begin{tabular}{l|llllll}
\toprule
\textbf{Party} & \textbf{caste1} & \textbf{odds of caste1} & \textbf{caste2} &  \textbf{Odds of caste2} &  \textbf{Odds Ratio} & \textbf{p-value} \\
\midrule
BJP  & \ucb & 0.329 &  \obc & 0.218 & 1.501 & 0.022 \\
 & \ucb & 0.329 & \scs & 0.154 & 2.136 & 0.016 \\
 & \ucnb & 0.522 & \ucb & 0.329 & 1.590 & 0.000 \\
 & \ucnb & 0.522 & \ic & 0.316 & 1.651 & 0.000 \\
 & \ucnb & 0.522 &  \obc & 0.218 & 2.397 & 0.000 \\
 & \ucnb & 0.522 & \scs & 0.154 & 3.396 & 0.000 \\
 & \ic & 0.316 & \scs & 0.154 & 2.057 & 0.028 \\
 & \st & 0.824 & \ucb & 0.329 & 2.507 & 0.012 \\ 
 & \st & 0.824 & \ic & 0.316 & 2.603 & 0.012 \\
 & \st & 0.824 & \obc  & 0.218 & 3.780 & 0.001\\
 & \st & 0.824 &  \scs  & 0.154 & 5.353 & 0.000 \\
  \bottomrule

Non-BJP &  \ucnb & 0.933 & \ucb & 0.344 & 2.715 & 0.042\\
& \ucnb & 0.933 & \obc & 0.337 & 2.771 & 0.015\\
& \ic & 0.944 & \ucb & 0.344 & 2.748 & 0.002 \\
& \ic & 0.944 & \obc & 0.337 & 2.804 & 0.000 \\
 & \ic & 0.944 & \oth & 0.475 & 1.990 & 0.028 \\
  & \scs & 2.400 & \ucb & 0.344 & 6.982 & 0.002\\
  & \scs & 2.400 & \obc & 0.337 & 7.125 & 0.000\\
  & \scs & 2.400 & \oth & 0.475 & 5.057 & 0.004\\
\bottomrule
\end{tabular}
}
\caption{\textbf{The second column, caste1, denotes the caste with higher odds of getting retweeted by their \textit{own} caste MPs than caste2 in fourth column. Odds ratio in the penultimate column is the proportion of odds of caste1 to that of caste2, and the last column denotes the p-value of the Fisher's exact test. The significance level is kept at 0.05 and all numbers are rounded to 3 decimal places}}
\label{table:samevsdiff}
\end{table}
